# Supplementary material for: Real-time Remote Tracking and Autonomous Planning for Whale Rendezvous using Robots
Source: arXiv:2512.05808 source file (2025-12-05)
Supplement: Supplementary file 1 [file appendix.tex]

\section{Appendix}
\subsection{Details of the VHF data and its evaluation} 
For the instance of data shown in Figure \ref{fig:vhf_ping_detection_from_tag}, the sperm whale performed shallow dives for approximately 4.5 hours, before performing a deep dive as shown in Figure \ref{fig:depth_profile_instance_nov_28}. Note that the depth sensor on the whale tag has noise and hence a reading of closer to 1 m indicates that the whale has likely surfaced.

As highlighted in Sec \ref{sec:Limitations}, VHF ping detection generated false positives for the first two hours due to another tag on the catamaran that was switched on. The raw data was collected at a sampling rate 2.048e6, but was downsampled by a factor of 16 to save for reproduction of the results. Later updates to the code that incorporated FFT, the sampling rate was reduced to 1.024e6 and downsampled by a factor of 8 due to technical issues related to regenerating results with FFT.  

Figure \ref{fig:signal_pulses_whale_tag} also highlights the constraint on VHF directionality computation when the tag is on the whale. The fishtracker on the whale tag transmits a pulse every second. Despite collecting data over 8 seconds, very few pulses are detectable using the current system. This is due to the fact that signal amplitude varies considerably due to bobbing motion of the whale and intermittent waves washing over the fishtracker (in contrast to Figure \ref{fig:vhf_ping_detection_range_test_samples} results which show the signal detection for a standalone tag floating over water) As such, directionality computation would require longer duration of data collection. Further works aims to leverage FFT for better pulse detection to minimize signal pulse loss.   

\begin{figure}
\centering
\includegraphics[scale=0.5]{Figures/RSS_2025_appendix_nov_28_complete_dive_profile.pdf}
% \vspace{-0.1 in}
\caption{Complete depth profile.}
\label{fig:depth_profile_instance_nov_28}
\end{figure}

\begin{figure}
\centering
\includegraphics[scale=0.5]{Figures/RSS_2025_appendix_nov_28_whale_tag_signal_pulses.pdf}
% \vspace{-0.1 in}
\caption{Signal pulse from tag on whale}
\label{fig:signal_pulses_whale_tag}
\end{figure}
